# Supplementary material for: Distance matters: the impact of gene proximity in bacterial gene regulation
Source: arXiv:1305.2677 source file (2013-05-13)
Supplement: Supplementary file 1 [file supp2.pdf]

# Supplementary Material
# Distance matters: the impact of gene proximity in bacterial gene regulation

Otto Pulkkinen[1] and Ralf Metzler[1,2]

[1]Department of Physics, Tampere University of Technology, FI-33101 Tampere, Finland
[2]Institute for Physics & Astronomy, University of Potsdam, D-14476 Potsdam-Golm, Germany

(Dated: 8th April 2013)

Here we present the explicit solution to the three-state model of operator dynamics that is depicted in magnifying glass **3** of Fig. 1, provide the expressions for parameters in the coarse-grained, telegraph noise scenario, and present stochastic simulations results for the mRNA numbers of the TF and TU genes. We also discuss the connection of our approach to the model of Kuhlman and Cox for intracellular transport of TFs.

The Markovian evolution of the full system is described by the set of differential equations

$$\begin{aligned}\frac{dp_b}{dt} &= -r_{bs}p_b + r_{sb}p_s\\ \frac{dp_s}{dt} &= -(r_{sb}+r_{su})p_s + r_{bs}p_b + r_{us}p_u\\ \frac{dp_u}{dt} &= -r_{us}p_u + r_{su}p_s\end{aligned} \tag{S1}$$

where $p_b$, $p_s$ and $p_u$ are the probabilities for the bound state, local search state, and unbound state, respectively. $r_{ij}$ is the transition rate from state $i$ to $j$ for $i,j=b,s,u$, and the rate of non-specific binding $r_{us}$ depends on the concentration of the repressor within the sliding distance from the operator. The solution of the linear system (S1), for given initial states $i=b,s,u$, is

$$\mathbf{p}(t|i) = \boldsymbol{\pi}_0 + C_+(i)e^{-\lambda_+ t}\boldsymbol{\pi}_+ + C_-(i)e^{-\lambda_- t}\boldsymbol{\pi}_-, \tag{S2}$$

where $\boldsymbol{\pi}_0$, $\boldsymbol{\pi}_+$ and $\boldsymbol{\pi}_-$ are the eigenvectors corresponding to eigenvalues $\lambda_0=0$ and

$$\begin{aligned}\lambda_\pm &= \pm\frac{1}{2}\sqrt{\left(\sum_{i\neq j} r_{ij}\right)^2 - 4(r_{us}r_{sb}+r_{us}r_{bs}+r_{su}r_{bs})}\\ &\quad +\frac{1}{2}\sum_{i\neq j} r_{ij}.\end{aligned} \tag{S3}$$

The coefficients $C_+$ and $C_-$ are found by setting $t=0$. The mean stationary transcription rate equals

$$\langle\alpha(t)\rangle_{st} = a(\pi_s+\pi_u) = \frac{a(r_{us}+r_{su})r_{bs}}{r_{us}r_{sb}+r_{us}r_{bs}+r_{su}r_{bs}}, \tag{S4}$$

and the stationary covariance becomes

$$\begin{aligned}C_{\rm st}(t) &= \langle\alpha(0)\alpha(t)\rangle_{\rm st} - \left(\langle\alpha(t)^2\rangle_{\rm st} - \langle\alpha(t)\rangle_{\rm st}^2\right)\\ &= a^2\left(B_+e^{-\lambda_+ t} + B_-e^{-\lambda_- t}\right),\end{aligned} \tag{S5}$$

where

$$B_\pm = \frac{\pm r_{bs}r_{sb}r_{us}}{r_{us}r_{sb}+r_{us}r_{bs}+r_{su}r_{bs}}\frac{\lambda_\mp(\lambda_\pm - r_{us} - r_{su})}{2\lambda_+ - \sum_{i\neq j} r_{ij}}. \tag{S6}$$

The mean number of proteins in a stationary state is

$$\langle M(\Omega,t)\rangle_{\rm st} = b\int_{-\infty}^{t}\langle\alpha(s)\rangle_{\rm st}\phi(\Omega,t-s)ds. \tag{S7}$$

For the variance at stationarity we also need the correlations of the transcription rate. From Eq. (4), we find

$$\begin{aligned}\langle M(\Omega,t)^2\rangle - \langle M(\Omega,t)\rangle^2 &= 2b^2\int_{-\infty}^{t}\langle\alpha(s)\rangle_{\rm st}\phi(\Omega,t-s)^2ds + b\int_{-\infty}^{t}\langle\alpha(s)\rangle_{\rm st}\left[1-\phi(\Omega,t-s)\right]\phi(\Omega,t-s)ds\\ &\quad +b^2\int_{-\infty}^{t}\int_{-\infty}^{t}C_{\rm st}(s-\tilde{s})\phi(\Omega,t-s)\phi(\Omega,t-\tilde{s})dsd\tilde{s}\end{aligned} \tag{S8}$$

For instance, if we are only interested in the total number of gene products in the cell, i.e., we consider $\phi(\text{Cell},t) = \exp(-\gamma t)$, we obtain the values

$$\langle M(t)\rangle_{\rm st} = \frac{b}{\gamma}\langle\alpha(t)\rangle_{\rm st},\ \ \langle M(t)^2\rangle_{\rm st} - \langle M(t)\rangle_{\rm st}^2 = \frac{b}{\gamma}\left(b+\frac{1}{2}\right)\langle\alpha(t)\rangle_{\rm st} + \frac{a^2b^2}{\gamma}\left(\frac{B_+}{\gamma+\lambda_+} + \frac{B_-}{\gamma+\lambda_-}\right) \tag{S9}$$

The first term in the variance contains the finite copy number fluctuations and protein bursts already present

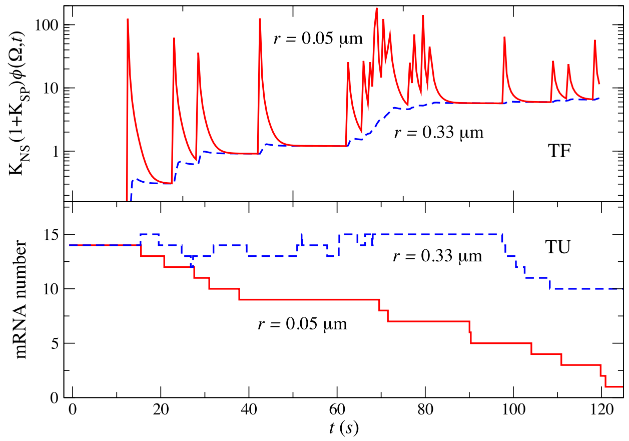


Figure S1: Sample time evolution of TF (repressor) density around the binding site (upper box) and the resulting TU mRNA numbers (lower box) in a simulation including stochastic production and degradation of the TF and TU mRNA with rate 1/(120sec), the TF, and their diffusion in the cell volume described by Eq. (9). The TU binding sites are at distances $r = 0.05$ $\mu$m (solid red lines) and $r = 0.33$ $\mu$m (blue dashed lines) from the TF gene. The number of transcripts of a close-by TU gene starts to decrease fast after the first emergence of TFs at $\approx$ 12sec, while the first repressor binding at a binding site further away occurs much later, $\approx$ 79sec.

in Eq. (6b). The new term originates from the operator state fluctuations.

The parameters of the coarse-grained model with telegraph operator noise are related to the parameters of the three-state model via the following relations obtained from solving the mean and the variance of the transcription rate,

$$a_{\rm eff} = a\left(1 - \frac{K_{\rm SP} r_{us}}{(1+K_{\rm SP})(r_{su}+r_{us})}\right) \quad \text{(S10a)}$$

$$r_{\rm on} = \frac{(r_{su}+r_{us})^2}{r_{su}(1+K_{\rm SP})+r_{us}} \quad \text{(S10b)}$$

$$r_{\rm off} = \frac{K_{\rm SP}^2 r_{su} r_{us}}{(1+K_{\rm SP})\left[r_{su}(1+K_{\rm SP})+r_{us}\right]}. \quad \text{(S10c)}$$

Fig. S1 shows results from stochastic simulations of the interacting TF and TU genes for the example of a repressing interaction. Note the distinct concentration peaks for close-by genes, and the fast decrement in expression level of the corresponding TU gene due to TF binding.

Kuhlman and Cox [Mol. Syst. Biol. **8**, 610 (2012)] also establish a model for intracellular transport of TFs. The cellular geometry is different from the one that we use in constructing the function $\phi(r,t)$ of Eqs. (8) and (9) in the main text. They approximate the nucleoid in an elongated cell by a one-dimensional line, which is in contact with a homogeneous pool of cytoplasm. However, both models share the idea of fast 3D diffusion in the cytoplasm, and an effective diffusion constant in the nucleoid. In particular, Kuhlman and Cox assume that, in the nucleoid, there are two species of TFs: those bound nonspecifically to the DNA and therefore performing a 1D sliding motion along it, and those diffusing freely in the space between DNA strands. We can make the same assumption in our model and write

$$\phi(r,t) = \phi_1(r,t) + \phi_3(r,t), \quad \text{(S11)}$$

where $\phi_1(r,t)$ and $\phi_3(r,t)$ are the densities of nonspecifically bound and freely diffusing TFs, respectively. Furthermore, assuming local equilibrium between these two species, we get

$$\phi_1(r,t) = K_{\rm NS}\cdot[DNA](r)\phi_3(r,t), \quad \text{(S12)}$$

where $[DNA](r)$ is the density of DNA at distance $r$ from the TF gene. Now the effective diffusion constant in the nucleoid reads

$$D_{\rm N} = \frac{D_1\phi_1(r,t)+D_3\phi_3(r,t)}{\phi(r,t)} = \frac{D_1 K_{\rm NS}[DNA](r)+D_3}{K_{\rm NS}[DNA](r)+1}. \quad \text{(S13)}$$

Taking $[DNA](r) \equiv [DNA] =$ constant for $r \leq R_N$ and zero elsewhere, we arrive to our model. As an example, giving an orders of magnitude impression, taking $[DNA] = 0.6$, $D_1 = 0.01\mu\text{m}^2/s$, $D_3 = 0.1\mu\text{m}^2/s$, and $K_{\rm NS} = 10$ yields $D_{\rm N} = 0.02\mu\text{m}^2/s$.
